# Supplementary material for: Upper bounds on the colloid separation efficiency of diffusiophoresis
Source: arXiv:2512.21758 source file (2026-05-10)
Supplement: Supplementary file 1 [file Separation_efficiency_of_diffusiophoresis_SI_v1.pdf]

# Supporting Information:

## Upper bounds on the separation efficiency of diffusiophoresis

Fernando Temprano-Coletto,<sup>†,‡</sup> Jeongmin Kim,<sup>†</sup> Marcel M. Louis,<sup>†</sup> and Howard A. Stone<sup>\*,†</sup>

<sup>†</sup> *Department of Mechanical and Aerospace Engineering, Princeton University, Princeton, NJ 08544, USA*

<sup>‡</sup> *Andlinger Center for Energy and the Environment, Princeton University, Princeton, NJ 08544, USA*

E-mail: hastone@princeton.edu

### Derivation of the leading-order particle profiles

#### Liquid sources

We start by combining the exact solution for the particle concentrations [Equation (19) in the main text] with the Taylor expansions for  $c_i$  for liquid sources [Equation (28) in the main text]. After factoring out  $c_i(0)$  from the numerator and denominator, and noting that the derivative at walls is negative at the source ( $dc_i/dy_+ < 0$  at  $y_+ = 0$ ) and positive at the sink ( $dc_i/dy_- > 0$  at  $y_- = 0$ ), we obtain

$$n_{\pm} = \frac{\left[1 \mp \frac{1}{c_i(0)} \left| \frac{dc_i}{dy_{\pm}}(0) \right| y_{\pm} + O(y_{\pm}^2) \right]^{\pm Pe_p}}{\int_0^1 \left[1 \mp \frac{1}{c_i(0)} \left| \frac{dc_i}{dy_{\pm}}(0) \right| y_{\pm} + O(y_{\pm}^2) \right]^{\pm Pe_p} dy_{\pm}}. \quad (\text{S1})$$

We then seek to find approximations for this expression at distances sufficiently close to the walls, where  $y_{\pm}$  is sufficiently small. To that end, we define  $y_{\pm} := \delta_{\pm} \xi_{\pm}$  as a rescaled wall coordinate, such that  $\xi_{\pm} = O(1)$  wherever  $y_{\pm} = O(\delta_{\pm})$ , and with  $\delta_{\pm}$  the (small) boundary layer thickness. This leads to

$$n_{\pm} = \frac{\left[1 \mp \frac{1}{c_i(0)} \left| \frac{dc_i}{dy_{\pm}}(0) \right| \delta_{\pm} \xi_{\pm} + O(\xi_{\pm}^2) \right]^{\pm Pe_p}}{\int_0^1 \left[1 \mp \frac{1}{c_i(0)} \left| \frac{dc_i}{dy_{\pm}}(0) \right| \delta_{\pm} \xi_{\pm} + O(\xi_{\pm}^2) \right]^{\pm Pe_p} d\xi_{\pm}}. \quad (\text{S2})$$

Since we expect a large absolute value of the exponent  $Pe_p \gg 1$ , we expect the terms of the expansion to be small if the boundary layer thickness is

$$\delta_{\pm} = \frac{c_i(0)}{\left| \frac{dc_i}{dy_{\pm}}(0) \right|} Pe_p^{-1}, \quad (\text{S3})$$

such that

$$n_{\pm} = \frac{\left[ 1 \mp \frac{\xi_{\pm}}{Pe_p} + O(Pe_p^{-2}) \right]^{\pm Pe_p}}{\delta_{\pm} \int_0^{1/\delta_{\pm}} \left[ 1 \mp \frac{\xi_{\pm}}{Pe_p} + O(Pe_p^{-2}) \right]^{\pm Pe_p} d\xi_{\pm}}. \quad (\text{S4})$$

Since the Péclet number is large, we can then invoke that  $\left[ 1 \mp \frac{\xi_{\pm}}{Pe_p} + O(Pe_p^{-2}) \right]^{\pm Pe_p} = e^{-\xi_{\pm}} [1 + O(Pe_p^{-1})]$  and, after integrating, obtain

$$n_{\pm} = \frac{e^{-\xi_{\pm}}}{\delta_{\pm} (1 - e^{-1/\delta_{\pm}})} + o(\delta_{\pm}^{-1}), \quad (\text{S5})$$

which, after neglecting exponentially small terms and changing variables back to  $y_{\pm}$ , results in

$$n_{\pm} = \frac{e^{-y_{\pm}/\delta_{\pm}}}{\delta_{\pm}} + o(\delta_{\pm}^{-1}), \quad (\text{S6})$$

whose leading-order term  $n_{\pm}^{(0)}$  is given by Equation (30a) in the main text.

## Gas sources

We can follow an analogous procedure combining the exact solution for the particles [Equation (19) in the main text] with the Taylor expansions for  $c_i$  for gas sources [Equation (29) in the main text]. After factoring out  $c_i(0)$  from the numerator and denominator, and noting that the second derivative at walls is negative at the source ( $d^2c_i/dy_+^2 < 0$  at  $y_+ = 0$ ) and positive at the sink ( $d^2c_i/dy_-^2 > 0$  at  $y_- = 0$ ), we obtain

$$n_{\pm} = \frac{\left[ 1 \mp \frac{1}{c_i(0)} \left| \frac{d^2c_i}{dy_{\pm}^2}(0) \right| \frac{y_{\pm}^2}{2} + O(y_{\pm}^3) \right]^{\pm Pe_p}}{\int_0^1 \left[ 1 \mp \frac{1}{c_i(0)} \left| \frac{d^2c_i}{dy_{\pm}^2}(0) \right| \frac{y_{\pm}^2}{2} + O(y_{\pm}^3) \right]^{\pm Pe_p} dy_{\pm}}. \quad (\text{S7})$$

Defining  $y_{\pm} := \delta_{\pm} \xi_{\pm}$  with a boundary layer thickness  $\delta_{\pm}$  such that

$$\delta_{\pm} = \left[ \frac{2c_i(0)}{\left| \frac{d^2 c_i}{dy_{\pm}^2}(0) \right|} \right]^{1/2} Pe_p^{-1/2}, \quad (\text{S8})$$

we obtain

$$n_{\pm} = \frac{\left[ 1 \mp \frac{\xi_{\pm}^2}{Pe_p} + O(Pe_p^{-2}) \right]^{\pm Pe_p}}{\delta_{\pm} \int_0^{1/\delta_{\pm}} \left[ 1 \mp \frac{\xi_{\pm}^2}{Pe_p} + O(Pe_p^{-2}) \right]^{\pm Pe_p} d\xi_{\pm}}. \quad (\text{S9})$$

After noting  $\left[ 1 \mp \frac{\xi_{\pm}^2}{Pe_p} + O(Pe_p^{-2}) \right]^{\pm Pe_p} = e^{-\xi_{\pm}^2} [1 + O(Pe_p^{-1})]$ , integrating, and neglecting exponentially small terms, we obtain

$$n_{\pm} = \frac{2e^{-\left(\frac{y_{\pm}}{\delta_{\pm}}\right)^2}}{\delta_{\pm} \sqrt{\pi}} + o(\delta_{\pm}^{-1}), \quad (\text{S10})$$

whose leading-order term  $n_{\pm}^{(0)}$  is given by Equation (30b) of the main text.

## Detailed asymptotics for the ionic concentration profiles

### Strong dissociation - Gas sources

Inserting the expansion  $c_i = c_i^{(0)} + Da_i c_i^{(1)} + O(Da_i^2)$  into Equation (23) of the main text, we obtain, at leading order,

$$\frac{d^4 c_i^{(0)}}{dy^4} = Da_s \frac{d^2 c_i^{(0)}}{dy^2}, \quad (\text{S11})$$

which has a solution

$$c_i^{(0)} = A + By + Ce^{-\sqrt{Da_s}y} + De^{\sqrt{Da_s}y}, \quad (\text{S12})$$

and with  $A, B, C, D$  constants. The boundary conditions given by (25) in the main text result in

$$\frac{d^2 c_i^{(0)}}{dy^2}(0) = \frac{d^2 c_i^{(0)}}{dy^2}(1) = \frac{dc_i^{(0)}}{dy}(0) = \frac{dc_i^{(0)}}{dy}(1) = 0 \quad (\text{S13})$$

at leading order, which give  $B = C = D = 0$  and  $c_i^{(0)} = A$ , with  $A$  undetermined.

At first order in  $Da_i$ , the governing equation is the same as in the zeroth-order case, i.e.

$$\frac{d^4 c_i^{(1)}}{dy^4} = Da_s \frac{d^2 c_i^{(1)}}{dy^2}, \quad (\text{S14})$$

with boundary conditions

$$\frac{d^2 c_i^{(1)}}{dy^2}(0) = \left(c_i^{(0)}\right)^\nu - 1 = A^\nu - 1 \quad \text{at } y = 0, \quad (\text{S15a})$$

$$\frac{d^2 c_i^{(1)}}{dy^2}(1) = \left(c_i^{(0)}\right)^\nu = A^\nu \quad \text{at } y = 1, \quad (\text{S15b})$$

$$\frac{dc_i^{(1)}}{dy}(0) = 0 \quad \text{at } y = 0, \quad (\text{S15c})$$

$$\frac{dc_i^{(1)}}{dy}(1) = 0 \quad \text{at } y = 1. \quad (\text{S15d})$$

The general solution of (S14) is  $c_i^{(1)} = E + Fy + Ge^{-\sqrt{Da_s}y} + He^{\sqrt{Da_s}y}$ , leaving five constants ( $A$ ,  $E$ ,  $F$ ,  $G$ , and  $H$ ) to be determined with only four boundary conditions (S15). However, an additional solvability condition can be determined integrating (S14) and imposing the no-flux conditions (S15c) and (S15d),

$$\begin{aligned} \int_0^1 \frac{d^4 c_i^{(1)}}{dy^4} dy &= Da_s \int_0^1 \frac{d^2 c_i^{(1)}}{dy^2} dy, \\ \frac{d^3 c_i^{(1)}}{dy^3}(1) - \frac{d^3 c_i^{(1)}}{dy^3}(0) &= Da_s \left[ \frac{dc_i^{(1)}}{dy}(1) - \frac{dc_i^{(1)}}{dy}(0) \right] = 0, \\ \frac{d^3 c_i^{(1)}}{dy^3}(1) &= \frac{d^3 c_i^{(1)}}{dy^3}(0). \end{aligned} \quad (\text{S16})$$

After solving for the constants, we obtain  $A = 2^{-1/\nu}$  and the solutions  $c_i^{(0)}$  and  $c_i^{(1)}$  given by Equations (36) in the main text.

## Weak dissociation - Liquid sources

Inserting the expansion  $c_i = c_i^{(0)} + Da_i^{-1}c_i^{(1)} + O(Da_i^{-2})$  into Equation (23) of the main text, we obtain

$$\frac{d^2}{dy^2} \left[ \left(c_i^{(0)}\right)^\nu \right] = 0, \quad (\text{S17a})$$

$$\frac{d^2}{dy^2} \left[ \nu \left(c_i^{(0)}\right)^{\nu-1} c_i^{(1)} \right] = \frac{d^4 c_i^{(0)}}{dy^4} - Da_s \frac{d^2 c_i^{(0)}}{dy^2}, \quad (\text{S17b})$$

at zeroth and first order, respectively, which have solutions given by

$$c_i^{(0)} = [A + By]^{1/\nu}, \quad (\text{S18a})$$

$$c_i^{(1)} = -\frac{B^2(\nu-1)}{\nu^3} [A + By]^{\frac{2-3\nu}{\nu}} - \frac{Da_s}{\nu} [A + By]^{\frac{2-\nu}{\nu}} + \frac{C + Dy}{\nu} [A + By]^{\frac{1-\nu}{\nu}}, \quad (\text{S18b})$$

However, these are only an “outer” solutions since they cannot satisfy all four boundary conditions given by (24) at each order simultaneously.

To find the solution close to the domain boundaries, we first introduce a rescaled “inner” coordinate  $y_B$  near the (bottom)  $y = 0$  wall, such that

$$y_B = Da_i^m y, \quad (\text{S19})$$

and introduce it into the governing equation (23) to obtain the inner equation

$$\frac{d^4 c_{iB}}{dy_B^4} = Da_i^{1-2m} \frac{d^2}{dy_B^2} [(c_{iB})^\nu] + Da_s Da_i^{-2m} \frac{d^2 c_{iB}}{dy_B^2}, \quad (\text{S20})$$

where we have denoted the inner solution as  $c_{iB}$  for notational convenience. The value  $m = 1/2$  is required to retain a meaningful dominant balance of terms, which leads to

$$\frac{d^4 c_{iB}}{dy_B^4} = \frac{d^2}{dy_B^2} [(c_{iB})^\nu] + Da_s Da_i^{-1} \frac{d^2 c_{iB}}{dy_B^2}, \quad (\text{S21})$$

which must be solved order by order imposing the boundary conditions at  $y_B = 0$  and matching to the outer solution as  $y_B \rightarrow \infty$ . To find out the terms in the matching, we expand the outer solution in the inner coordinate  $y_B$  as

$$\begin{aligned} c_i(y_B) &= c_i^{(0)}(y_B) + Da_i^{-1} c_i^{(1)}(y_B) + O(Da_i^{-2}) = \\ &= [A + Da_i^{-1/2} B y_B]^{1/\nu} + Da_i^{-1} c_i^{(1)}(y_B) + O(Da_i^{-2}) = \\ &= A^{1/\nu} + Da_i^{-1/2} \frac{A^{1-\nu}}{\nu} B y_B + Da_i^{-1} \left[ -\frac{A^{1-2\nu}}{2\nu^2} B^2(\nu-1) y_B^2 + c_i^{(1)}(y_B = 0) \right] + O(Da_i^{-3/2}). \end{aligned} \quad (\text{S22})$$

We then pose an expansion of the inner solution  $c_{iB} = c_{iB}^{(0)} + Da_i^{-1/2} c_{iB}^{(1)} + Da_i^{-1} c_{iB}^{(2)} + O(Da_i^{-3/2})$  and insert it in the inner equation (S21) and in the boundary conditions to obtain the inner problem at each order.

At zeroth order, we have

$$\frac{d^4 c_{iB}^{(0)}}{dy_B^4} = \frac{d^2}{dy_B^2} \left[ \left( c_{iB}^{(0)} \right)^\nu \right], \quad (\text{S23a})$$

$$c_{iB}^{(0)} = 1 \text{ at } y_B = 0, \quad (\text{S23b})$$

$$\frac{d^2 c_{iB}^{(0)}}{dy_B^2} = 0 \text{ at } y_B = 0, \quad (\text{S23c})$$

$$c_{iB}^{(0)} \rightarrow A^{1/\nu} \text{ as } y_B \rightarrow \infty, \quad (\text{S23d})$$

which requires the constant to be  $A = 1$  and results in  $c_{iB}^{(0)} = 1$ .

At order  $Da_i^{-1/2}$ , we find

$$\frac{d^4 c_{iB}^{(1)}}{dy_B^4} = \nu \frac{d^2 c_{iB}^{(1)}}{dy_B^2}, \quad (\text{S24a})$$

$$c_{iB}^{(1)} = 0 \text{ at } y_B = 0, \quad (\text{S24b})$$

$$\frac{d^2 c_{iB}^{(1)}}{dy_B^2} = 0 \text{ at } y_B = 0, \quad (\text{S24c})$$

$$c_{iB}^{(1)} \rightarrow \frac{B}{\nu} y_B \text{ as } y_B \rightarrow \infty, \quad (\text{S24d})$$

which has solution  $c_{iB}^{(1)} = \frac{B}{\nu} y_B$ .

At order  $Da_i^{-1}$ , we find

$$\frac{d^4 c_{iB}^{(2)}}{dy_B^4} = \nu \frac{d^2}{dy_B^2} \left[ \frac{(\nu - 1)B^2}{2\nu^2} y_B^2 + c_{iB}^{(2)} \right], \quad (\text{S25a})$$

$$c_{iB}^{(2)} = 0 \text{ at } y_B = 0, \quad (\text{S25b})$$

$$\frac{d^2 c_{iB}^{(2)}}{dy_B^2} = 0 \text{ at } y_B = 0, \quad (\text{S25c})$$

$$c_{iB}^{(2)} \rightarrow -\frac{(\nu - 1)B^2}{2\nu^2} y_B^2 \text{ as } y_B \rightarrow \infty, \quad (\text{S25d})$$

which has solution  $c_{iB}^{(2)} = \frac{(\nu - 1)B^2}{\nu^3} \left[ e^{-\sqrt{\nu} y_B} - \frac{\nu}{2} y_B^2 - 1 \right]$ .

We can then proceed analogously with the boundary-layer analysis of the (top)  $y = 1$  wall. Introducing a rescaled “inner” coordinate  $y_T$  such that

$$y_T = Da_i^{1/2} (1 - y), \quad (\text{S26})$$

and plugging it into Equation (23) of the main text, we obtain the inner equation

$$\frac{d^4 c_{iT}}{dy_T^4} = \frac{d^2}{dy_T^2} [(c_{iT})^\nu] + Da_s Da_i^{-1} \frac{d^2 c_{iT}}{dy_T^2}. \quad (\text{S27})$$

Expanding the outer solution in the inner coordinate  $y_T$ , we arrive at

$$\begin{aligned} c_i(y_T) &= c_i^{(0)}(y_T) + Da_i^{-1} c_i^{(1)}(y_T) + O(Da_i^{-2}) = \\ &= [(1+B) - Da_i^{-1/2} B y_T]^{1/\nu} + Da_i^{-1} c_i^{(1)}(y_T) + O(Da_i^{-2}) = \\ &= (1+B)^{1/\nu} - Da_i^{-1/2} \frac{B(1+B)^{\frac{1-\nu}{\nu}}}{\nu} y_T + \\ &\quad + Da_i^{-1} \left[ -\frac{(\nu-1)B^2(1+B)^{\frac{1-2\nu}{\nu}}}{2\nu^2} y_T^2 + c_i^{(1)}(y_T=0) \right] + O(Da_i^{-3/2}), \end{aligned} \quad (\text{S28})$$

where we have already used  $A = 1$  obtained from the matching conditions at the bottom  $y = 0$  boundary.

Then, we insert an expansion of the inner solution  $c_{iT} = c_{iT}^{(0)} + Da_i^{-1/2} c_{iT}^{(1)} + Da_i^{-1} c_{iT}^{(2)} + O(Da_i^{-3/2})$  in the inner equation (S27) and in the boundary conditions to obtain the inner problem at each order.

At zeroth order, we have

$$\frac{d^4 c_{iT}^{(0)}}{dy_T^4} = \frac{d^2}{dy_T^2} \left[ (c_{iT}^{(0)})^\nu \right], \quad (\text{S29a})$$

$$c_{iT}^{(0)} = \varepsilon^{1/\nu} \text{ at } y_T = 0, \quad (\text{S29b})$$

$$\frac{d^2 c_{iT}^{(0)}}{dy_T^2} = 0 \text{ at } y_T = 0, \quad (\text{S29c})$$

$$c_{iT}^{(0)} \rightarrow (1+B)^{1/\nu} \text{ as } y_T \rightarrow \infty, \quad (\text{S29d})$$

which requires the constant to be  $B = \varepsilon - 1$  and results in  $c_{iT}^{(0)} = \varepsilon^{1/\nu}$ .

At order  $Da_i^{-1/2}$ , we find

$$\frac{d^4 c_{iT}^{(1)}}{dy_T^4} = \nu \varepsilon^{\frac{\nu-1}{\nu}} \frac{d^2 c_{iT}^{(1)}}{dy_T^2}, \quad (\text{S30a})$$

$$c_{iT}^{(1)} = 0 \text{ at } y_T = 0, \quad (\text{S30b})$$

$$\frac{d^2 c_{iT}^{(1)}}{dy_T^2} = 0 \text{ at } y_T = 0, \quad (\text{S30c})$$

$$c_{iT}^{(1)} \rightarrow \frac{(1-\varepsilon)\varepsilon^{\frac{1-\nu}{\nu}}}{\nu} y_T \text{ as } y_T \rightarrow \infty, \quad (\text{S30d})$$

with solution  $c_{iT}^{(1)} = \frac{(1-\varepsilon)\varepsilon^{\frac{1-\nu}{\nu}}}{\nu} y_T$ .

At order  $Da_i^{-1}$ , we find

$$\frac{d^4 c_{iT}^{(1)}}{dy_T^4} = \nu \varepsilon^{\frac{\nu-1}{\nu}} \frac{d^2}{dy_T^2} \left[ \frac{(\nu-1)(1-\varepsilon)^2 \varepsilon^{\frac{1-2\nu}{\nu}}}{2\nu^2} y_T^2 + c_{iT}^{(2)} \right], \quad (\text{S31a})$$

$$c_{iT}^{(2)} = 0 \text{ at } y_T = 0, \quad (\text{S31b})$$

$$\frac{d^2 c_{iT}^{(2)}}{dy_T^2} = 0 \text{ at } y_T = 0, \quad (\text{S31c})$$

$$c_{iT}^{(2)} \rightarrow -\frac{(\nu-1)(1-\varepsilon)^2 \varepsilon^{\frac{1-2\nu}{\nu}}}{2\nu^2} y_T^2 \text{ as } y_T \rightarrow \infty, \quad (\text{S31d})$$

which has solution  $c_{iT}^{(2)} = \frac{(\nu-1)(1-\varepsilon)^2 \varepsilon^{\frac{2-3\nu}{\nu}}}{\nu^3} \left[ e^{-\sqrt{\nu\varepsilon^{\frac{\nu-1}{2\nu}}} y_T} - \frac{\nu\varepsilon^{\frac{\nu-1}{\nu}}}{2} y_T^2 - 1 \right]$ .

In summary, the solutions near the bottom and top walls can then be expressed as

$$c_{iB} = 1 - Da_i^{-1/2} \frac{(1-\varepsilon)}{\nu} y_B + Da_i^{-1} \frac{(\nu-1)(1-\varepsilon)^2}{\nu^3} \left[ e^{-\sqrt{\nu} y_B} - \frac{\nu}{2} y_B^2 - 1 \right] + O\left(Da_i^{-3/2}\right), \quad (\text{S32a})$$

$$c_{iT} = \varepsilon^{1/\nu} - Da_i^{-1/2} \frac{(1-\varepsilon)\varepsilon^{\frac{1-\nu}{\nu}}}{\nu} y_T + Da_i^{-1} \frac{(\nu-1)(1-\varepsilon)^2 \varepsilon^{\frac{2-3\nu}{\nu}}}{\nu^3} \left[ e^{-\sqrt{\nu\varepsilon^{\frac{\nu-1}{2\nu}}} y_T} - \frac{\nu\varepsilon^{\frac{\nu-1}{\nu}}}{2} y_T^2 - 1 \right] + O\left(Da_i^{-3/2}\right), \quad (\text{S32b})$$

which can be re-expressed in terms of the outer variables  $y_+ = Da_i^{1/2} y_B$  and  $y_- = Da_i^{1/2} y_T$  and then expanded up to linear order to obtain

$$c_i \approx 1 - \frac{(1-\varepsilon)}{\nu} \left[ 1 + Da_i^{-1/2} \frac{(\nu-1)(1-\varepsilon)}{\nu^{3/2}} \right] y_+ \quad \text{at the source}, \quad (\text{S33a})$$

$$c_i \approx \varepsilon^{1/\nu} + \frac{(1-\varepsilon)\varepsilon^{\frac{1-\nu}{\nu}}}{\nu} \left[ 1 - Da_i^{-1/2} \frac{(\nu-1)(1-\varepsilon)\varepsilon^{\frac{1-3\nu}{2\nu}}}{\nu^{3/2}} \right] y_- \quad \text{at the sink}. \quad (\text{S33b})$$

After neglecting terms of order  $Da_i^{-1/2}$ , the above expressions (S33) simplify into Equations (39) in the main text. It is worth remarking that, since  $\nu > 1$  and  $0 < \varepsilon < 1$ , the  $O\left(Da_i^{-1/2}\right)$  term in (S33a) can always be neglected for sufficiently large  $Da_i \gg 1$ . However, the expression  $\varepsilon^{\frac{1-3\nu}{2\nu}}$  could become large if  $\varepsilon \ll 1$ , potentially compensating the small  $Da_i^{-1/2}$  and invalidating the asymptotic expansion. This breakdown of the theory stems from the implicit assumption that  $\varepsilon = O(1)$ . Since a more careful analysis for a small  $\varepsilon \ll 1$  would be out of the scope of this paper, we simply remark that the theory will be valid as long as

$$Da_i \gg \frac{(\nu-1)^2}{\nu^3} (1-\varepsilon)^2 \varepsilon^{\frac{1-3\nu}{\nu}}, \quad (\text{S34})$$

under which the  $O(Da_i^{-1/2})$  term in (S33b) can clearly be safely neglected.

## Weak dissociation - Gas sources

In the case of gas sources, the only difference with respect to the liquid sources is the boundary conditions. Therefore, we also pose an expansion  $c_i = c_i^{(0)} + Da_i^{-1} c_i^{(1)} + O(Da_i^{-2})$ , insert it in Equation (23) of the main text, and obtain the same outer solutions

$$c_i^{(0)} = [A + By]^{1/\nu}, \quad (\text{S35a})$$

$$c_i^{(1)} = -\frac{B^2(\nu-1)}{\nu^3} [A + By]^{\frac{2-3\nu}{\nu}} - \frac{Da_s}{\nu} [A + By]^{\frac{2-\nu}{\nu}} + \frac{C + Dy}{\nu} [A + By]^{\frac{1-\nu}{\nu}}, \quad (\text{S35b})$$

at zeroth and first order, respectively. Note that these are identical to the outer solution for the case of a liquid source (S18).

To find the inner solution close to the bottom  $y = 0$  boundary, we introduce the same rescaled “inner” coordinate  $y_B$  near the (bottom)  $y = 0$  wall as in the case for liquid sources, such that

$$y_B = Da_i^{1/2} y, \quad (\text{S36})$$

which, once introduced in the governing equation (23), leads to a hierarchy of inner problems analogous to those of the case with liquid sources (S23) and (S24), with the same matching conditions but with different boundary conditions at the bottom wall  $y_B = 0$ .

At zeroth order, the inner problem is

$$\frac{d^4 c_{iB}^{(0)}}{dy_B^4} = \frac{d^2}{dy_B^2} \left[ \left( c_{iB}^{(0)} \right)^\nu \right], \quad (\text{S37a})$$

$$\left( c_{iB}^{(0)} \right)^\nu - \frac{d^2 c_{iB}^{(0)}}{dy_B^2} = 1 \text{ at } y_B = 0, \quad (\text{S37b})$$

$$\frac{dc_{iB}^{(0)}}{dy_B} = 0 \text{ at } y_B = 0, \quad (\text{S37c})$$

$$c_{iB}^{(0)} \rightarrow A^{1/\nu} \text{ as } y_B \rightarrow \infty, \quad (\text{S37d})$$

which leads to  $A = 1$  and to a solution  $c_{iB}^{(0)} = 1$ .

At order  $Da_i^{-1/2}$ , the inner problem is

$$\frac{d^4 c_{iB}^{(1)}}{dy_B^4} = \nu \frac{d^2 c_{iB}^{(1)}}{dy_B^2}, \quad (\text{S38a})$$

$$c_{iB}^{(1)} - \frac{d^2 c_{iB}^{(1)}}{dy_B^2} = 0 \text{ at } y_B = 0, \quad (\text{S38b})$$

$$\frac{d^1 c_{iB}^{(1)}}{dy_B^1} = 0 \text{ at } y_B = 0, \quad (\text{S38c})$$

$$c_{iB}^{(1)} \rightarrow \frac{B}{\nu} y_B \text{ as } y_B \rightarrow \infty, \quad (\text{S38d})$$

which has solution  $c_{iB}^{(1)} = \frac{B}{\nu} \left[ y_B + \frac{e^{-\sqrt{\nu} y_B}}{\nu^{1/2}} \right]$ .

To find the inner solution close to the top  $y = 1$  boundary, we need a different boundary layer rescaling, since a naive  $y_T = Da_i^{1/2}(1 - y)$  fails to produce a consistent leading-order inner problem. The reason for this is that, unlike the case of a liquid source where  $c_i(y = 1) \rightarrow \varepsilon$  as  $Da_i \rightarrow \infty$ , for a gas source we have that  $c_i(y = 1) \rightarrow 0$  as  $Da_i \rightarrow \infty$ , and therefore  $c_i(y = 1)$  can get arbitrarily small and must also be rescaled by a small parameter to arrive at a consistent inner problem. We therefore pose a scaling

$$y_T = Da_i^m (1 - y), \quad (\text{S39a})$$

$$c_{iT} = Da_i^n c_i, \quad (\text{S39b})$$

which, introduced in Equation (23) of the main text, leads to

$$\frac{d^4 c_{iT}}{dy_T^4} = Da_i^{1-2m-(\nu-1)n} \frac{d^2}{dy_T^2} [(c_{iT})^\nu] + Da_s Da_i^{-2m} \frac{d^2 c_{iT}}{dy_T^2}. \quad (\text{S40})$$

Similarly, this rescaling turns the boundary conditions (25b) and (25c) of the main text into

$$Da_i^{1-2m-(\nu-1)n} c_{iT}^\nu - \frac{d^2 c_{iT}}{dy_T^2} = 0, \quad (\text{S41a})$$

$$\frac{dc_{iT}}{dy_T} = 0. \quad (\text{S41b})$$

We therefore set

$$n = \frac{1 - 2m}{\nu - 1} \quad (\text{S42})$$

to achieve a meaningful dominant balance. We can then determine the value of  $m$  by examining the matching condition: expressing the outer solution in terms of the inner variable  $y_T$  and noting that  $A = 1$  from the

previous analysis, we obtain

$$c_i(y_T) = [(1 + B) - Da_i^{-m} B y_T]^{1nu} + O(Da_i^{-1}). \quad (\text{S43})$$

The matching condition dictates that, if  $B \neq 0$ , the inner solution must satisfy  $Da_i^{-n} c_{iT} \rightarrow (1 + B)^{1\nu}$  as  $y_T \rightarrow \infty$  at leading order. This condition can be satisfied with  $n = 0$ , which reverts to  $m = 1/2$  and the naive scaling  $y_T = Da_i^{1/2}(1 - y)$ , and to an leading order problem given by

$$\frac{d^4 c_{iT}^{(0)}}{dy_T^4} = \frac{d^2}{dy_T^2} \left[ \left( c_{iT}^{(0)} \right)^\nu \right], \quad (\text{S44a})$$

$$c_{iT}^\nu - \frac{d^2 c_{iT}}{dy_T^2} = 0 \text{ at } y_T = 0, \quad (\text{S44b})$$

$$\frac{dc_{iT}^{(0)}}{dy_T} = 0 \text{ at } y_T = 0, \quad (\text{S44c})$$

$$c_{iT}^{(0)} \rightarrow (1 + B)^{1/\nu} \text{ as } y_T \rightarrow \infty, \quad (\text{S44d})$$

which only admits a solution if  $B = -1$ , which contradicts our prior assumption. The only option left is then that  $B = -1$  but  $n \neq 0$ , in which case the outer solution can be expanded as

$$c_i(y_T) = Da_i^{-m/\nu} y_T^{1/\nu} + O(Da_i^{-1}). \quad (\text{S45})$$

The leading-order matching condition at leading order is then  $Da_i^{-n} c_{iT} \rightarrow Da_i^{-m/\nu} y_T^{1/\nu}$  as  $y_T \rightarrow \infty$ , which requires  $m = \nu n$ . In combination with the previous condition of  $n = (1 - 2m)/(\nu - 1)$ , this leads to

$$m = \frac{\nu}{3\nu - 1}, \quad (\text{S46a})$$

$$n = \frac{1}{3\nu - 1}, \quad (\text{S46b})$$

with values tabulated in Table S1.

Table S1: Values of the exponents  $m$  and  $n$  in Equation (S46) for different values of  $\nu$ .

| $\nu$ | 2   | 3   | 4    | 5    |
|-------|-----|-----|------|------|
| $m$   | 2/5 | 3/8 | 4/11 | 5/14 |
| $n$   | 1/5 | 1/8 | 1/11 | 1/14 |

With these exponents, we arrive at the zeroth-order inner problem

$$\frac{d^4 c_{iT}^{(0)}}{dy_T^4} = \frac{d^2}{dy_T^2} \left[ \left( c_{iT}^{(0)} \right)^\nu \right], \quad (\text{S47a})$$

$$c_{iT}^\nu - \frac{d^2 c_{iT}}{dy_T^2} = 0 \text{ at } y_T = 0, \quad (\text{S47b})$$

$$\frac{dc_{iT}^{(0)}}{dy_T} = 0 \text{ at } y_T = 0, \quad (\text{S47c})$$

$$c_{iT}^{(0)} \rightarrow y_T^{1/\nu} \text{ as } y_T \rightarrow \infty, \quad (\text{S47d})$$

which can be integrated twice to yield

$$\frac{d^2 c_{iT}^{(0)}}{dy_T^2} = \left( c_{iT}^{(0)} \right)^\nu - y_T, \quad (\text{S48a})$$

$$\frac{dc_{iT}^{(0)}}{dy_T} = 0 \quad \text{at } y_T = 0, \quad (\text{S48b})$$

$$c_{iT}^{(0)} \rightarrow y_T^{1/\nu} \quad \text{as } y_T \rightarrow \infty. \quad (\text{S48c})$$

As opposed to all the cases outlined above, this problem is nonlinear and does not, in general, have an exact solution. In the particular case of  $\nu = 2$ , the problem can be mapped to the so-called first Painlevé transcendent<sup>S1</sup> after a change of variables. This problem has been shown to lack exact solutions in terms of elementary functions so, in order to find a local expansion of its solution, we pose a Taylor series

$$c_{iT}^{(0)} = \alpha + \beta y_T^2 + O(y_T^3), \quad (\text{S49})$$

introduce it in (S48), and obtain  $\beta = \alpha^\nu/2$ , and where the parameter  $\alpha = c_{iT}(0)$  must be calculated by numerically solving (S48).

In summary, the solutions near the bottom and top walls can then be expressed as

$$c_{iB} = 1 - \frac{Da_i^{-1/2}}{\nu} \left[ y_B + \frac{e^{-\sqrt{\nu}y_B}}{\nu^{1/2}} \right] + O(Da_i^{-1}), \quad (\text{S50a})$$

$$c_{iT} = \alpha + \frac{\alpha^\nu}{2} y_T^2 + O(y_T^3). \quad (\text{S50b})$$

Changing coordinates to  $y_+ = Da_i^{-1/2} y_B$  and  $y_- = Da_i^{-\frac{\nu}{3\nu-1}} y_T$  and rescaling, the expansions of the solution

near the walls can be obtained as

$$c_{iB} \approx \left[ 1 - \frac{Da_i^{-1/2}}{\nu^{3/2}} \right] - Da_i^{-1/2} \frac{y_+^2}{2\nu^{1/2}} \quad \text{at the source,} \quad (\text{S51a})$$

$$c_{iT} \approx Da_i^{-\frac{1}{3\nu-1}} \alpha + Da_i^{\frac{2\nu-1}{3\nu-1}} \frac{\alpha^\nu}{2} y_-^2 \quad \text{at the sink,} \quad (\text{S51b})$$

which coincide with Equations (42) from the main text.

## Calibration of particle fluorescence intensity

In order to corroborate that the measured fluorescence intensity is proportional to the particle concentration, we run calibration tests in which particle suspensions at different volume fractions are driven through the same experimental setup, but without the injection of  $\text{CO}_2$  or  $\text{N}_2$  gases. This causes the particle distribution to remain homogeneous with the known volume fraction introduced through the inlet. Plots of the fluorescent signal as a function of the volume fraction are presented in Figure S1.

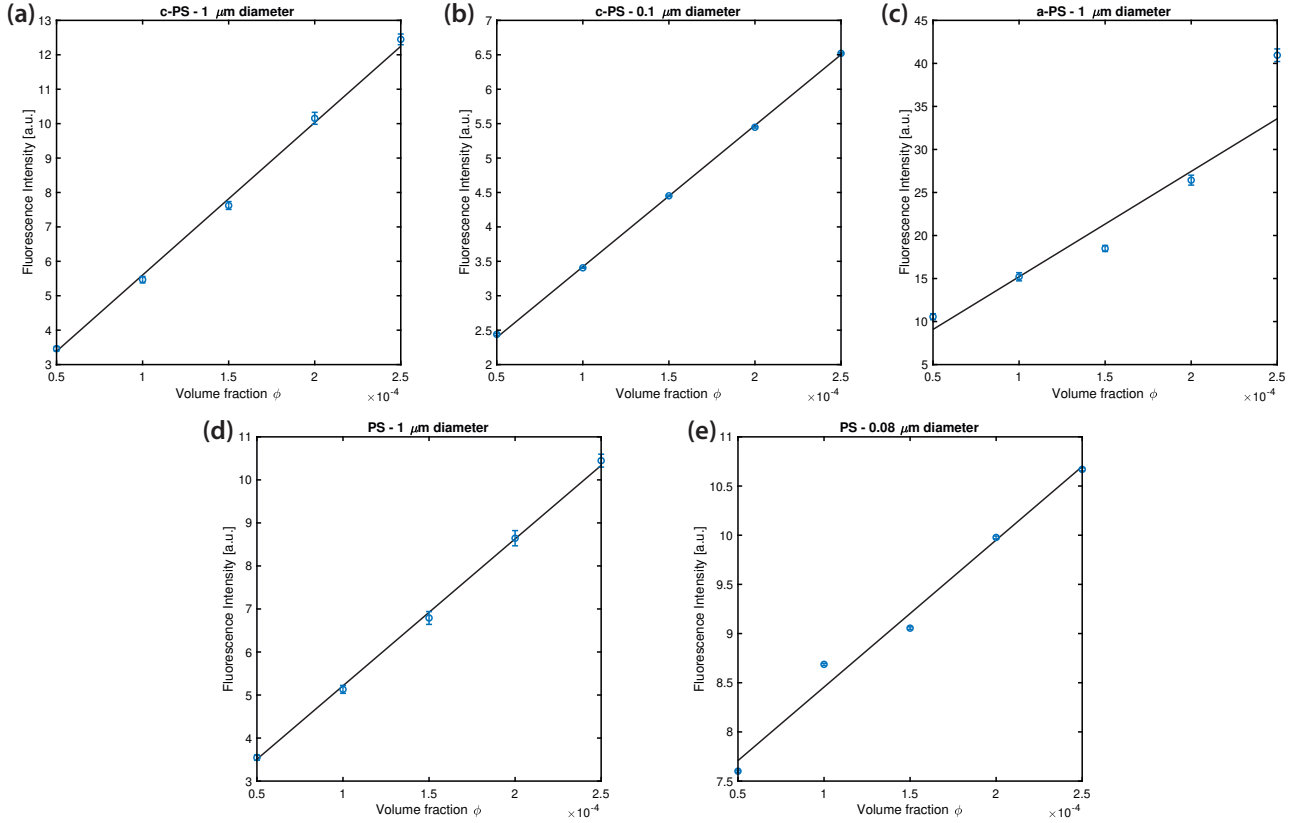

Figure S1: Fluorescence calibration tests for five particle types and sizes. The error bars indicate the standard deviation resulting from averaging the fluorescence signal in time,  $X$ , and  $Y$  for each calibration test. The black line corresponds to a linear least-squares fit weighted by the standard deviations.

## References

- (S1) Bender, C. M.; Orszag, S. A. *Advanced mathematical methods for scientists and engineers I: Asymptotic methods and perturbation theory*; Springer, New York, NY, 1999.
